# Supplementary material for: Bound states in the continuum and Fano resonances in the strong mode coupling regime
Source: arXiv:1805.09265 ancillary file (2018-12-01)
Supplement: Supplementary file 1 [file supplemental_v0.pdf]

# Supplemental materials:
# Bound states in the continuum and Fano resonances in the strong mode coupling regime

Andrey A. Bogdanov[1,2], Kirill L. Koshelev[1,3], Polina V. Kapitanova[1], Mikhail V. Rybin[1,2],
Sergey A. Gladyshev[1], Zarina F. Sadrieva[1], Kirill B. Samusev[1,2], Yuri S. Kivshar[1,3], and Mikhail F. Limonov[1,2]
[1]*ITMO University, St. Petersburg 197101, Russia*
[2]*Ioffe Institute, St. Petersburg 194021, Russia and*
[3]*Nonlinear Physics Centre, Australian National University, Canberra ACT 2601, Australia*

In the Supplemental Materials we (i) derive the Fano formula for the scattering cross section for a lossless resonator, (ii) provide details on splitting of the open resonator into the closed part and the radiation continuum and (iii) derive Equations 5(a) and 5(b) of the main text.

## I. DERIVATION OF THE FANO FORMULA FOR THE SCATTERING CROSS SECTION FOR A LOSSLESS RESONATOR

We study the scattering cross section (SCS) of a disk resonator characterized by isotropic dielectric permittivity $\varepsilon(\omega, \mathbf{r})$. The resonator is lossless which implies that absorption is zero at the frequency region of interest. The incident wave is a linearly polarized plane wave $\mathbf{E}_{\rm inc}$

$$\mathbf{E}_{\rm inc}(\omega, \mathbf{r}) = \mathbf{E}_0 \exp{(i\mathbf{k}_{\rm inc} \cdot \mathbf{r})}, \tag{1}$$

where the amplitude $\mathbf{E}_0$ is real.

The scattering cross section $\sigma$ is equal to the extinction cross section. We apply the optical theorem to calculate the extinction cross section?

$$\sigma = \frac{4\pi c}{\omega \mathbf{E}_0^2} \mathrm{Im} \left[ \mathbf{E}_0 \cdot \hat{\mathbf{E}}_{\rm sc}(\mathbf{n}_{\rm inc}) \right], \tag{2}$$

where $\hat{\mathbf{E}}_{\rm sc}(\mathbf{n}_{\rm inc})$ is the amplitude of scattered field in the direction of the incident wave.

The scattered field satisfies the Lippmann-Schwinger equation?

$$\mathbf{E}_{\rm sc}(\mathbf{r}) = -\frac{\omega^2}{c^2} \int d\mathbf{r}^{'}\ \Delta\epsilon(\omega, \mathbf{r}^{'}) \hat{\mathbf{G}}_{\rm f}(\omega, \mathbf{r}, \mathbf{r}^{'}) \cdot \left[ \mathbf{E}_{\rm inc}(\omega, \mathbf{r}^{'}) + \mathbf{E}_{\rm sc}(\mathbf{r}^{'}) \right], \tag{3}$$

where $\hat{\mathbf{G}}_{\rm f}$ is the free space dyadic Green's function.

The amplitude of the far-field distribution of $\hat{\mathbf{G}}_{\rm f}$ in the direction of incident field is given by

$$\hat{\mathbf{G}}_{\rm f}(\omega, \mathbf{n}_{\rm inc}, \mathbf{r}^{'}) = -\left[ \hat{I} - \mathbf{n}_{\rm inc} \otimes \mathbf{n}_{\rm inc} \right] \frac{\exp{[-i\mathbf{k}_{\rm inc} \cdot \mathbf{r}^{'})]}}{4\pi}. \tag{4}$$

Substitution of Eq. 3 and Eq. 4 into Eq. 2 gives

$$\sigma = \frac{1}{\mathbf{E}_0^2} \mathrm{Im} \left\{ \frac{\omega}{c} \int d\mathbf{r}^{'}\ \Delta\epsilon(\omega, \mathbf{r}^{'}) \mathbf{E}^*_{\rm inc}(\omega, \mathbf{r}^{'}) \cdot \left[ \mathbf{E}_{\rm inc}(\omega, \mathbf{r}^{'}) + \mathbf{E}_{\rm sc}(\mathbf{r}^{'}) \right] \right\}. \tag{5}$$

Analysis of Eq. 5 shows that the scattered field in the right side of the equation is evaluated only inside the resonator. Therefore, $\mathbf{E}_{\rm sc}$ can be expanded over the eigenmodes (the resonant states) of the system $\mathbf{E}_j$, as they form the complete basis inside the scatterer?

$$\mathbf{E}_{\rm sc}(\mathbf{r}) = -\omega \sum_j \frac{\mathbf{E}_j(\mathbf{r})}{2(\omega - \omega_j)} \int d\mathbf{r}^{'}\ \Delta\epsilon(\omega, \mathbf{r}^{'}) \mathbf{E}_j(\mathbf{r}^{'}) \cdot \mathbf{E}_{\rm inc}(\omega, \mathbf{r}^{'}). \tag{6}$$

Since the disk resonator posses inversion symmetry, each resonant state can be classified with respect to the inversion symmetry as $\mathbf{E}_j(-\mathbf{r}) = (-1)^p \mathbf{E}_j(\mathbf{r})$, where $p = 0, 1$ is the parity defining even or odd resonant state, respectively. Expanding $\mathbf{E}_{\rm sc}$ over the resonant states by means of Eq. 6 and using the inversion symmetry properties allows to reduce the expression for the SCS

$$\sigma = \frac{c^2}{\omega^2 \mathbf{E}_0^2} \mathrm{Im} \left\{ C(\omega) - c \sum_j \frac{(-1)^p \kappa_j(\omega)^2}{2(\omega - \omega_j)} \right\}. \tag{7}$$

Here

$$C(\omega) = \frac{\omega^3}{c^3}\int d\mathbf{r}^{'}\ \Delta\epsilon(\omega,\mathbf{r}^{'})|\mathbf{E}_{\rm inc}(\omega,\mathbf{r}^{'})|^2, \tag{8}$$

$$\kappa_j(\omega) = -\frac{\omega^2}{c^2}\int d\mathbf{r}^{'}\ \Delta\epsilon(\omega,\mathbf{r}^{'})\mathbf{E}_j(\mathbf{r}^{'})\cdot\mathbf{E}_{\rm inc}(\omega,\mathbf{r}^{'}). \tag{9}$$

We focus on frequencies in the vicinity of the eigenfrequency $\omega_0 - i\gamma$ of the particular resonant state with index $j_0$ and parity $p_0$. Then, SCS can be written as

$$\sigma = \frac{c^2}{\omega^2\mathbf{E}_0^2}\left[B_1(\omega) + \mathrm{Im}\left\{\frac{B_2(\omega)}{\Omega + i}\right\}\right], \tag{10}$$

where the coefficients are determined below

$$B_1(\omega) = \mathrm{Im}\left\{C(\omega) - c\sum_{j\neq j_0}\frac{(-1)^p\kappa_j^2(\omega)}{2(\omega-\omega_j)}\right\}, \tag{11}$$

$$B_2(\omega) = \frac{[i^{1+p_0}\kappa(\omega)]^2}{2\gamma/c}, \tag{12}$$

$$\Omega = \frac{\omega-\omega_0}{\gamma}. \tag{13}$$

Finally, the we reduce Eq. 10 to the conventional Fano formula

$$\sigma = \frac{c^2}{\omega^2\mathbf{E}_0^2}\left[\frac{A(\omega)}{1+q^2(\omega)}\frac{(q(\omega)+\Omega)^2}{1+\Omega^2} + I_{\rm bg}(\omega)\right]. \tag{14}$$

Here the Fano parameters are

$$q(\omega) = -\cot\left[\Delta(\omega)\right], \tag{15}$$

$$\Delta(\omega) = (p_0-1)\pi/2 + \arg\left[\kappa(\omega)\right], \tag{16}$$

$$A(\omega) = |B_2(\omega)| = \frac{|\kappa(\omega)|^2}{2\gamma/c}, \tag{17}$$

$$I_{\rm bg}(\omega) = B_1(\omega) - \frac{|B_2(\omega)|}{1+q^2(\omega)}. \tag{18}$$

In the vicinity of $\omega_0$ the frequency dependence of $A(\omega)$, $q(\omega)$ and $I_{\rm bg}(\omega)$ is smooth and can be neglected.

Importantly, in the main manuscript we focus on the avoided resonance crossing between the $\mathrm{TE}_{1,1,0}$ and $\mathrm{TM}_{1,1,1}$ modes. Both modes are odd with respect to inversion symmetry, which means that $p_0 = 1$ and $\Delta(\omega) = \arg\left[\kappa(\omega)\right]$.

## II. SPLITTING OF THE OPEN RESONATOR INTO THE CLOSED PART AND THE RADIATION CONTINUUM.

In this section we show how the resonant state can be treated as the eigenmode of a closed resonator interacting with the radiation continuum. The most rigorous approach is based on the Fano-Feshbach projection scheme[?] . However, here we apply another method based on the perturbation theory.

We study an open electromagnetic resonator. We focus on the particular resonant state $\mathbf{E}_{\rm rs}$. We enclose the resonator with a spherical boundary, which is placed in the far field of the resonant state and is characterized by the normal $\mathbf{n}$. While radiation losses are weak, the resonant state can be divided into sum

$$\mathbf{E}_{\rm rs}(\mathbf{r}) = \mathbf{E}^{(0)}(\mathbf{r}) + i\delta\mathbf{E}(\mathbf{r}), \tag{19}$$

where $\mathbf{E}^{(0)}(\mathbf{r})$ is the solution of Maxwell's equations inside the spherical shell with perfect magnetic boundary conditions

$$\mathbf{n}\times\nabla\times\mathbf{E}^{(0)} = 0. \tag{20}$$

We study the modes with high quality factor more than 10, therefore, $\delta\mathbf{E}(\mathbf{r})$ is the first order perturbation of $\mathbf{E}^{(0)}(\mathbf{r})$ and can be treated as a real-valued function, while other corrections of the perturbation theory are neglected.

The resonant state is normalised as[?]

$$1=\int_V dV\,\varepsilon\mathbf{E}_{\rm rs}\cdot\mathbf{E}_{\rm rs}+\frac{c^2}{2\omega_{\rm rs}^2}\oint_S dS\left[\mathbf{E}_{\rm rs}\cdot\frac{\partial}{\partial r}r\frac{\partial\mathbf{E}_{\rm rs}}{\partial r}-r\left(\frac{\partial\mathbf{E}_{\rm rs}}{\partial r}\right)^2\right], \tag{21}$$

where both volume and surface integration goes over the spherical shell which was introduced before.

Boundary conditions Eq. 20 imply that for $\mathbf{E}^{(0)}(\mathbf{r})$ the surface integral in Eq. 21 is zero and the normalization within the zero order of the perturbation theory is

$$1=\int_V dV\,\varepsilon\mathbf{E}^{(0)}\cdot\mathbf{E}^{(0)}. \tag{22}$$

For each resonant state $\mathbf{E}_{\rm rs}$ with complex frequency $\omega_{\rm rs}=\omega_0-i\gamma$ the another resonant state with frequency $-\omega_0-i\gamma$ and field $\mathbf{E}^*_{\rm rs}$ must exist in the spectrum of an open system. We can find the elegant formula for damping rate $\gamma$ by exploiting the orthogonality condition between these complementary resonant states

$$0=[\omega_{\rm rs}^2-(\omega_{\rm rs}^*)^2]\int_V dV\,\varepsilon\mathbf{E}_{\rm rs}\cdot\mathbf{E}^*_{\rm rs}-c^2\oint_S dS\left[\mathbf{E}_{\rm rs}\cdot\frac{\partial\mathbf{E}^*_{\rm rs}}{\partial r}-\mathbf{E}^*_{\rm rs}\cdot\frac{\partial\mathbf{E}_{\rm rs}}{\partial r}\right]. \tag{23}$$

Since the surface $S$ is located in the far field, we can use the relation $\partial\mathbf{E}_{\rm rs}/\partial r=i\omega_{\rm rs}/c\,\mathbf{E}_{\rm rs}$ and simplify Eq. 23 to the form

$$2\frac{\gamma}{c}=\frac{\oint_S dS|\mathbf{E}_{\rm rs}|^2}{\int_V dV\,\varepsilon|\mathbf{E}_{\rm rs}|^2}. \tag{24}$$

Within the first order perturbation theory Eq. 24 is reduced to

$$2\frac{\gamma}{c}=\oint_S dS|\mathbf{E}_{\rm rs}|^2. \tag{25}$$

To calculate the surface integral we apply the Lippmann-Schwinger equation to the resonant state itself

$$\mathbf{E}_{\rm rs}(\mathbf{r})=-\frac{\omega_{\rm rs}^2}{c^2}\int d\mathbf{r}'\,\Delta\epsilon(\omega_{\rm rs},\mathbf{r}')\hat{\mathbf{G}}_{\rm f}(\omega_{\rm rs},\mathbf{r},\mathbf{r}')\cdot\mathbf{E}_{\rm rs}(\mathbf{r}'). \tag{26}$$

Using the perturbation theory it can be transformed to

$$\mathbf{E}_{\rm rs}(\mathbf{r})=-\frac{\omega_0^2}{c^2}\int d\mathbf{r}'\,\Delta\epsilon(\omega_0,\mathbf{r}')\hat{\mathbf{G}}_{\rm f}(\omega_0,\mathbf{r},\mathbf{r}')\cdot\mathbf{E}_{\rm rs}(\mathbf{r}'). \tag{27}$$

Finally, we expand the free space Green's function $\hat{\mathbf{G}}_{\rm f}$ into outer product of the vector spherical waves $\mathbf{E}_\alpha$, which represent the set of independent channels of the radiation continuum[?]

$$\hat{\mathbf{G}}_{\rm f}(\omega_0,\mathbf{r},\mathbf{r}')=i\frac{\omega_0}{c}\sum_\alpha\mathbf{E}_\alpha(\omega_0,\mathbf{r})\otimes\mathbf{E}_\alpha(\omega_0,\mathbf{r}'). \tag{28}$$

Now we substitute Eq. 27 and Eq. 28 into Eq. 25 and perform the surface integration. Since vector spherical harmonics are orthogonal on a unit sphere and the boundary $S$ is located in the far field of the resonant state, we arrive at Eq.4 of the main text

$$2\frac{\gamma}{c}=\sum_\alpha|\mathrm{D}_\alpha|^2. \tag{29}$$

Here the coupling amplitudes $\mathrm{D}_\alpha$ are

$$\mathrm{D}_\alpha=-\frac{\omega_0^2}{c^2}\int d\mathbf{r}'\,\Delta\epsilon(\omega_0,\mathbf{r}')\mathbf{E}_\alpha(\omega_0,\mathbf{r}')\cdot\mathbf{E}_{\rm rs}(\mathbf{r}'). \tag{30}$$

## III. ANALYSIS OF THE COUPLING COEFFICIENT $\kappa$

In this section we derive Eq.5(a-b) of the main text. We start from the definition of $\kappa$ given in Eq. 9. We decompose the incident wave $\mathbf{E}_{\rm inc}$ into the vector spherical waves

$$\mathbf{E}_{\rm inc}(\omega, \mathbf{r}) = \sum_{\alpha} s_{\alpha} \mathbf{E}_{\alpha}(\omega, \mathbf{r}). \tag{31}$$

Then the coupling coefficient can be also decomposed into contribution of radiation channels as

$$\kappa(\omega) = \sum_{\alpha} s_{\alpha} \mathrm{D}_{\alpha}(\omega). \tag{32}$$

Importantly, in the main manuscript we focus on the avoided resonance crossing between the $\mathrm{TE}_{1,1,0}$ and $\mathrm{TM}_{1,1,1}$ modes. These modes have azimuthal index $n = 1$ which means that they interact only with channels with the same azimuthal index. Straightforward analysis shows that for this particular case all relevant coefficients $s_{\alpha}$ are real-valued and have nearly the same magnitude (only few channels with close indices give contribution to the scattering). Therefore, $\Delta = \arg(\kappa)$ is determined only by the interference between the phases of $\mathrm{D}_{\alpha}$. Since $\mathrm{D}_{\alpha} = \mathrm{D}_{\alpha}^{(0)} + i\delta\mathrm{D}_{\alpha}$ and both $\mathrm{D}_{\alpha}^{(0)}$ and $\delta\mathrm{D}_{\alpha}$ are real-valued (because we work within the first order of the perturbation theory) the phase $\Delta$ takes critical values when

$$\sum_{\alpha} \delta\mathrm{D}_{\alpha} = 0, \qquad \Delta = 0, \tag{33}$$

$$\sum_{\alpha} \mathrm{D}_{\alpha}^{(0)} = 0, \qquad \Delta = \pi/2. \tag{34}$$

These equations are equivalent to Eq.5(a-b) of the main text.
